# Supplementary material for: Random Offset Block Embedding Array (ROBE) for CriteoTB Benchmark MLPerf DLRM Model : 1000$\times$ Compression and 3.1$\times$ Faster Inference
Source: arXiv:2108.02191 source file (2022-01-22)
Supplement: Supplementary file 1 [file appendix_theory.tex]

\subsection{Theory}
\subsubsection{Analysis of projection of embedding-table as a parameter vector (single vector containing all embedding paramters) onto the memory - A feature hashing style evaluation of projection}
The quality of the inner product estimate is one of the key metrics to understand the quality of space approximation while performing dimensionality reduction. Let us analyse the inner product of projection we discussed in the \rma-Z. Consider a vectors of size n which is projected using \rma-Z. Let us consider the inner product. In this analysis we also consider that each element is added to the location with a sign hash function $g$. In our case we are mapping the entire embedding flattened out row-wise and all embedding tables are concatenated into a single vector of size n : which is number of parameters in the original (or virtual / simulated) embedding tables. Let the size of the reduced dimension be $m$. In our case that is equal to the size of the memory $m = |M|$. Let the chunk size be Z. Let the memory allocation function be h.

Let $x \in R^n$ and $y \in R^n$
\begin{equation}
    \widehat{\ip{x}{y}} = \ip{x}{y} + \Sigma_{i \neq j}  x_i y_j \mathcal{I}(h(i) {==} h(j)) g(i) g(j)
\end{equation}
Let $\mathcal{C}_i$ be the chunk-id that is assigned to to i, following the same notation used in equations \ref{eq:eq_rmax} 
Then
we know for sure that $\mathcal{I}(h(i) {==} h(j))$ is 0 if $\mathcal{C}_i {==} \mathcal{C}_j$
Using this fact.
\begin{equation}
    \widehat{\ip{x}{y}} = \ip{x}{y} + \Sigma_{\mathcal{C}_i \neq \mathcal{C}_j}  x_i y_j \mathcal{I}(h(i) {==} h(j)) g(i) g(j)
\end{equation}
We can easily see that this estimator of $\ip{x}{y}$ is unbiased.
Let us now look at the 

\begin{equation}
    \mathbb{E}(\hat{\ip{x}{y}}) = \ip{x}{y}
\end{equation}

The variance of the estimator can be computed as 
\begin{equation}
    \mathbb{V}(\hat{\ip{x}{y}}) = \mathbb{E}((\Sigma_{\mathcal{C}_i \neq \mathcal{C}_j}  x_i y_j \mathcal{I}(h(i) {==} h(j)) g(i) g(j))^2)
\end{equation}
Using the fact that $\mathbb{E}(g(i)) = 0$, we can simplify the expression above
\begin{equation}
    \mathbb{V}(\hat{\ip{x}{y}}) = \frac{1}{m-Z+1} (\Sigma_{\mathcal{C}_i \neq \mathcal{C}_j}  x_i^2 y_j^2 +  \Sigma_{\mathcal{C}_i \neq \mathcal{C}_j} x_i y_i x_j y_j) \label{eq:var}
\end{equation}

Note that when Z=1, the equation for variance is exactly the random projection that is used for "feature hashing" as proposed by Charrikar et. al.
Substituting for $\mathcal{C}_i$, we have 

\begin{equation}
    \mathbb{V}(\hat{\ip{x}{y}}) = \frac{1}{m-Z+1} (\Sigma_{\mathcal{C}_i \neq \mathcal{C}_j}  x_i^2 y_j^2 +  \Sigma_{i//Z \neq j//Z} x_i y_i x_j y_j)
\end{equation}
Even if m is of the order of 1M , which is 4MB, we only choose Z to be at max the bus size which is like 32 or 64. Hence, note that this variance is not very different from the variance when Z=1.
We can further simplify the expression as follows. Let $\mathbb{V}_Z(x,y,n)$ be the variance of inner product of x and y : vectors of dimension n while using the \rma-Z. Then we can write the expression as

\begin{equation}
 \mathbb{V}_Z(x, y, n) = \frac{m}{m - Z + 1} (\mathbb{V}_1(x,y,n) - \Sigma_{\mathcal{C}_i} \mathbb{V}_1(x_{\mathcal{C}_i},y_{\mathcal{C}_i},Z)) 
\end{equation}
where $x_{\mathcal{C}_i}$ is a subvector of with dimension Z which lies in a chunk.

It would be an interesting endeavour to check how does the variance $\mathbb{V}_Z$, $Z > 1$ compares to $\mathbb{V}_1$.
So lets look at $\mathbb{V}_Z - \mathbb{V}_1$

\begin{equation}
 \mathbb{V}_Z(x, y, n) - \mathbb{V}_1(x,y,n)= \frac{m}{m - Z + 1} (\mathbb{V}_1(x,y,n) - \Sigma_{\mathcal{C}_i} \mathbb{V}_1(x_{\mathcal{C}_i},y_{\mathcal{C}_i},Z)) - \mathbb{V}_1(x,y,n)
\end{equation}
\begin{equation}
 \mathbb{V}_Z(x, y, n) - \mathbb{V}_1(x,y,n)= \frac{1}{m - Z + 1} ((Z-1) \mathbb{V}_1(x,y,n) - m \Sigma_{\mathcal{C}_i} \mathbb{V}_1(x_{\mathcal{C}_i},y_{\mathcal{C}_i},Z))
\end{equation}
\begin{equation}
 \mathbb{V}_Z(x, y, n) - \mathbb{V}_1(x,y,n)= \frac{\mathbb{V}_1}{m - Z + 1} ((Z-1) - m \frac{\Sigma_{\mathcal{C}_i} \mathbb{V}_1(x_{\mathcal{C}_i},y_{\mathcal{C}_i},Z)}{\mathbb{V}_1(x,y,n)})
\end{equation}
Now it can be seen that for any arbitrary x, y there is no certain relation between $\mathbb{V}_Z$ and $\mathbb{V}_1$. So let us make some assumption on data that can cover most of the datasets and still help us draw some conclusion on how $\mathbb{V}_Z$ relates to $\mathbb{V}_1$

Using the equations \ref{eq:var}, we can see that $\Sigma_{\mathcal{C}_i} \mathbb{V}_1(x_{\mathcal{C}_i},y_{\mathcal{C}_i},Z)$ we have $\frac{n}{Z} (Z(Z-1) = n(Z-1)$ terms both of the form $x_i^2 y_j^2$ and $x_iy_ix_jy_j$. Similarly in $V_1(x,y,n)$ we have $n(n-1)$ terms of the same forms.
Let's assume that $\mu_1 = E(x_i^2 y_j^2)$ and  $\mu_2 = E(x_iy_ix_jy_j)$ is similar in numerator and denominator. Essentially, we are assuming that these terms are of similar magnitude. If there is a weird skew in these terms the variance relation can go on either sides.

\begin{equation}
 \mathbb{V}_Z(x, y, n) - \mathbb{V}_1(x,y,n)= \frac{\mathbb{V}_1}{m - Z + 1} ((Z-1) - m \frac{n(Z-1) (\mu_1 + \mu_2)}{n(n-1) (\mu_1 + \mu_2})
\end{equation}

\begin{equation}
 \mathbb{V}_Z(x, y, n) - \mathbb{V}_1(x,y,n)= \frac{\mathbb{V}_1 (Z-1)}{m - Z + 1} (1 -  \frac{m}{(n-1)})
\end{equation}

\begin{equation}
 \frac{\mathbb{V}_Z(x, y, n) - \mathbb{V}_1(x,y,n)}{\mathbb{V}_1(x,y,n)} = \frac{\frac{(Z-1)}{m}}{1 - \frac{(Z - 1)}{m}} (1 - \frac{m}{(n-1)})
\end{equation}

Let us use $\alpha = \frac{Z-1}{m}$ and $\beta = \frac{m}{n-1}$
\begin{equation}
 \frac{\mathbb{V}_Z(x, y, n) - \mathbb{V}_1(x,y,n)}{\mathbb{V}_1(x,y,n)} = \frac{\alpha}{1 - \alpha} (1 - \beta)\label{eq:var_final}
\end{equation}

\begin{figure}[h]
    \centering
    \includegraphics[scale=0.25]{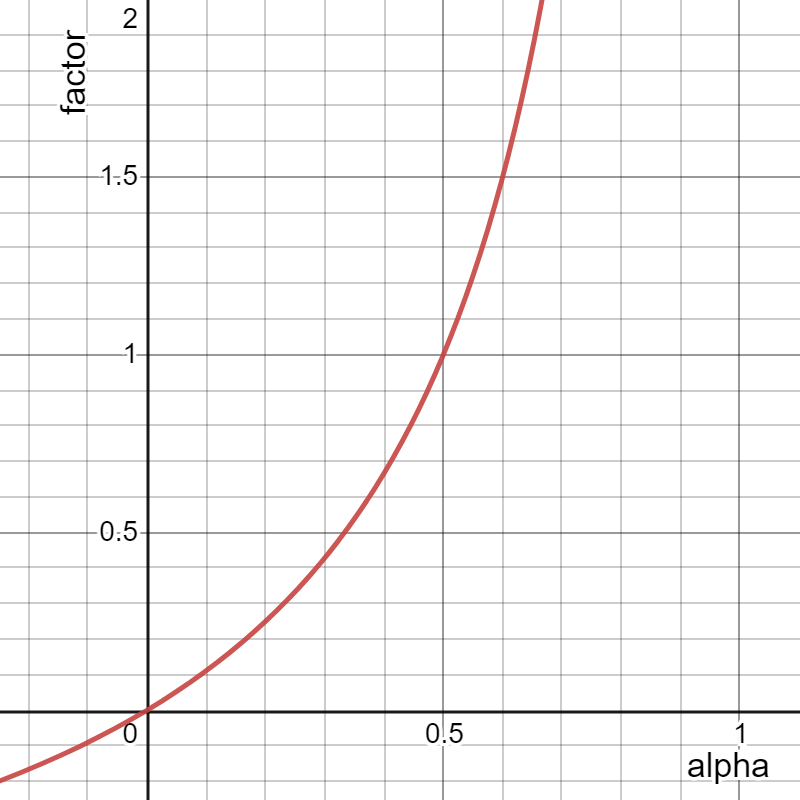}
    \caption{RHS of equation \ref{eq:var_final}}
    \label{fig:perf1}
\end{figure}

Note that the Z is of the order of 0-64, while m is generally in the range of $10^5$ and even beyond! In fact $m = 10^6$ just means 4MB memory.
So $Z << m$ and at such a small value we can simple approximate the expression with 

Let us use $\alpha = \frac{Z-1}{m}$ and $\beta = \frac{m}{n-1}$
\begin{equation}
 \frac{\mathbb{V}_Z(x, y, n) - \mathbb{V}_1(x,y,n)}{\mathbb{V}_1(x,y,n)} \approx \alpha (1 - \beta) < \alpha \quad \quad [ \textrm{ when } Z << m ]
\end{equation}
In most realistic settings $\alpha < 10^{-6}$

\subsection{Effect of \rma-Z on inner product of embeddings of two values - i.e. parts of parameter vector that are identified as two separate embeddings. }

The previous analysis was the analysis of the sketching matrix and how good it is in preserving distances in a space. However, another important aspect of this projection - pertinent to the discussion of this paper is how does this projection of entire parameter vector affect the inter- embedding relation between embeddings of two different values. 

Consider how the parameter vector is constructed. We flatten out each embedding table row wise ( so each embedding is contiguous) and we concatenate all flattened embedding tables together to get a single parameter vector which is projected down.
Let each embedding has a dimension of $d$ and $Z$ divides $d$. The parameter vector, $\theta$, with length $n$, of course, i s divisible by $Z$ and $d$ both.
Without loss of generality, let us consider the embeddings $x = \theta_{1:d}$ and $y = \theta_{(d+1):2d}$. 

Lets look at the product of two elements first $\theta_1 \theta_{(d+1)}$

\begin{equation}
    \hat{\theta_1} = \sum_{i=1}^n \theta_i g(1) g(i) \mathcal{I}(h(i) == h(1))
\end{equation}

Hence,
\begin{equation}
    \widehat{\theta_1 \theta_{(d+1)}} = \sum_{i=1}^n  \sum_{j=1}^n \theta_i \theta_j g(1) g(i) g(d+1) g(j) \mathcal{I}(h(i) == h(1)) \mathcal{I}(h(j) == h(d+1))
\end{equation}

\begin{equation}
\begin{split}
    &\widehat{\theta_1 \theta_{(d+1)}} = \theta_1 \theta_{(d+1)} + \\
    &\sum_{i=1, \mathcal{C}(i) \neq \mathcal{C}(1) }^n  \sum_{j=1, \mathcal{C}(j) \neq \mathcal{C}(d+1)}^n \theta_i \theta_j g(1) g(i) g(d+1) g(j) \mathcal{I}(h(i) == h(1)) \mathcal{I}(h(j) == h(d+1))
\end{split}
\end{equation}

The expected value of above equation is non zero only when either $(i == 1, j == d+1)$  or $(i==d+1, j==1)$. Also d+1 and 1 can collide as they lie in separate chunks.  Hence we have 

\begin{equation}
    \mathbb{E}(\widehat{\theta_1 \theta_{(d+1)}}) = \theta_1 \theta_{(d+1)} (1 + \frac{1}{m})
\end{equation}
Also, we have
\begin{equation}
    \ip{x}{y} = \sum_{k=1}^d \theta_k \theta_{(d+k)}
\end{equation}

\begin{equation}
    \widehat{\ip{x}{y}} = \sum_{k=1}^d \sum_{i=1}^n  \sum_{j=1}^n \theta_i \theta_j g(k) g(i) g(d+k) g(j) \mathcal{I}(h(i) == h(k)) \mathcal{I}(h(j) == h(d+k))
\end{equation}

\begin{equation}
\begin{split}
    & \widehat{\ip{x}{y}} =  \ip{x}{y} + \\
    &\sum_{k=1}^d \sum_{i=1, \mathcal{C}(i) \neq \mathcal{C}(k) }^n  \sum_{j=1, \mathcal{C}(j) \neq \mathcal{C}(d+k)}^n \theta_i \theta_j g(k) g(i) g(d+k) g(j) \mathcal{I}(h(i) == h(k)) \mathcal{I}(h(j) == h(d+k))
\end{split}
\end{equation}

Hence,
\begin{equation}
    \mathbb{E}(\widehat{\ip{x}{y}}) = \mathbb{E}(\widehat{\ip{\theta_{1:d}}{\theta_{(d+1):2d}}}) = \ip{x}{y} (1 + \frac{1}{m - Z + 1})
\end{equation}

\begin{equation}
    \mathbb{V}(\widehat{\ip{x}{y}}) = \mathbb{E}\left((\sum_{k=1}^d \sum_{i=1, \mathcal{C}(i) \neq \mathcal{C}(k) }^n  \sum_{j=1, \mathcal{C}(j) \neq \mathcal{C}(d+k)}^n \theta_i \theta_j g(k) g(i) g(d+k) g(j) \mathcal{I}(h(i) == h(k)) \mathcal{I}(h(j) == h(d+k)))^2\right)
\end{equation}

\begin{equation}
\begin{split}
    &\mathbb{V}(\widehat{\ip{x}{y}}) = \mathbb{E} \\ &  ((\sum_{k=1}^d \quad \sum_{i=1, \mathcal{C}(i) \neq \mathcal{C}(k) }^n  \quad \sum_{j=1, \mathcal{C}(j) \neq \mathcal{C}(d+k)}^n  \quad  \sum_{k'=1}^d \quad \sum_{i'=1, \mathcal{C}(i') \neq \mathcal{C}(k') }^n  \quad  \sum_{j'=1, \mathcal{C}(j') \neq \mathcal{C}(d + k')}^n \\
    & \quad \quad \theta_i \theta_j  \theta_{i'} \theta_{j'} \\
    & \quad \quad g(k) g(i) g(d+k) g(j) g(k') g(i') g(d+k') g(j')\\
    & \quad \quad \mathcal{I}(h(i) == h(k)) \mathcal{I}(h(j) == h(d+k))  \mathcal{I}(h(i') == h(k')) \mathcal{I}(h(j') == h(d+k')) ) )\\
    \end{split}
\end{equation}

\begin{equation}
\begin{split}
    &\mathbb{V}(\widehat{\ip{x}{y}}) = \mathbb{E} \\ &  ((\sum_{k=1}^d \quad \sum_{i=1, \mathcal{C}(i) \neq \mathcal{C}(k) }^n  \quad \sum_{j=1, \mathcal{C}(j) \neq \mathcal{C}(d+k)}^n  \quad  \sum_{k'=1}^d \quad \sum_{i'=1, \mathcal{C}(i') \neq \mathcal{C}(k') }^n  \quad  \sum_{j'=1, \mathcal{C}(j') \neq \mathcal{C}(d + k')}^n \\
    & \quad \quad \theta_i \theta_j  \theta_{i'} \theta_{j'} \\
    & \quad \quad g(k) g(i) g(d+k) g(j) g(k') g(i') g(d+k') g(j')\\
    & \quad \quad \mathcal{I}(h(i) == h(k)) \mathcal{I}(h(j) == h(d+k))  \mathcal{I}(h(i') == h(k')) \mathcal{I}(h(j') == h(d+k')) ) )\\
    \end{split}
\end{equation}
