# Supplementary material for: Random Offset Block Embedding Array (ROBE) for CriteoTB Benchmark MLPerf DLRM Model : 1000$\times$ Compression and 3.1$\times$ Faster Inference
Source: arXiv:2108.02191 source file (2022-01-22)
Supplement: Supplementary file 2 [file appendix_theory_throwaway.tex]

\textbf{CASE : $Z < d$}

Let each embedding has a dimension of $d$ and $Z$ divides $d$. The parameter vector, $\theta$, with length $n$, of course, i s divisible by $Z$ and $d$ both.
Without loss of generality, let us consider the embeddings $x = \theta_{1:d}$ and $y = \theta_{(d+1):2d}$. 

Lets look at the product of two elements first $\theta_1 \theta_{(d+1)}$

\begin{equation}
    \hat{\theta_1} = \sum_{i=1}^n \theta_i g(1) g(i) \mathcal{I}(h(i) == h(1))
\end{equation}

Hence,
\begin{equation}
    \widehat{\theta_1 \theta_{(d+1)}} = \sum_{i=1}^n  \sum_{j=1}^n \theta_i \theta_j g(1) g(i) g(d+1) g(j) \mathcal{I}(h(i) == h(1)) \mathcal{I}(h(j) == h(d+1))
\end{equation}

\begin{equation}
\begin{split}
    &\widehat{\theta_1 \theta_{(d+1)}} = \theta_1 \theta_{(d+1)} + \\
    &\sum_{i=1, \mathcal{C}(i) \neq \mathcal{C}(1) }^n  \sum_{j=1, \mathcal{C}(j) \neq \mathcal{C}(d+1)}^n \theta_i \theta_j g(1) g(i) g(d+1) g(j) \mathcal{I}(h(i) == h(1)) \mathcal{I}(h(j) == h(d+1))
\end{split}
\end{equation}

The expected value of above equation is non zero only when either $(i == 1, j == d+1)$  or $(i==d+1, j==1)$. Also d+1 and 1 can collide as they lie in separate chunks.  Hence we have 

\begin{equation}
    \mathbb{E}(\widehat{\theta_1 \theta_{(d+1)}}) = \theta_1 \theta_{(d+1)} (1 + \frac{1}{m})
\end{equation}
Also, we have
\begin{equation}
    \ip{x}{y} = \sum_{k=1}^d \theta_k \theta_{(d+k)}
\end{equation}

\begin{equation}
    \widehat{\ip{x}{y}} = \sum_{k=1}^d \sum_{i=1}^n  \sum_{j=1}^n \theta_i \theta_j g(k) g(i) g(d+k) g(j) \mathcal{I}(h(i) == h(k)) \mathcal{I}(h(j) == h(d+k))
\end{equation}

\begin{equation}
\begin{split}
    & \widehat{\ip{x}{y}} =  \ip{x}{y} + \\
    &\sum_{k=1}^d \sum_{i=1, \mathcal{C}(i) \neq \mathcal{C}(k) }^n  \sum_{j=1, \mathcal{C}(j) \neq \mathcal{C}(d+k)}^n \theta_i \theta_j g(k) g(i) g(d+k) g(j) \mathcal{I}(h(i) == h(k)) \mathcal{I}(h(j) == h(d+k))
\end{split}
\end{equation}

Hence,
\begin{equation}
    \mathbb{E}(\widehat{\ip{x}{y}}) = \mathbb{E}(\widehat{\ip{\theta_{1:d}}{\theta_{(d+1):2d}}}) = \ip{x}{y} (1 + \frac{1}{m - Z + 1})
\end{equation}

\begin{equation}
    \mathbb{V}(\widehat{\ip{x}{y}}) = \mathbb{E}\left((\sum_{k=1}^d \sum_{i=1, \mathcal{C}(i) \neq \mathcal{C}(k) }^n  \sum_{j=1, \mathcal{C}(j) \neq \mathcal{C}(d+k)}^n \theta_i \theta_j g(k) g(i) g(d+k) g(j) \mathcal{I}(h(i) == h(k)) \mathcal{I}(h(j) == h(d+k)))^2\right)
\end{equation}

\begin{equation}
\begin{split}
    &\mathbb{V}(\widehat{\ip{x}{y}}) = \mathbb{E} \\ &  ((\sum_{k=1}^d \quad \sum_{i=1, \mathcal{C}(i) \neq \mathcal{C}(k) }^n  \quad \sum_{j=1, \mathcal{C}(j) \neq \mathcal{C}(d+k)}^n  \quad  \sum_{k'=1}^d \quad \sum_{i'=1, \mathcal{C}(i') \neq \mathcal{C}(k') }^n  \quad  \sum_{j'=1, \mathcal{C}(j') \neq \mathcal{C}(d + k')}^n \\
    & \quad \quad \theta_i \theta_j  \theta_{i'} \theta_{j'} \\
    & \quad \quad g(k) g(i) g(d+k) g(j) g(k') g(i') g(d+k') g(j')\\
    & \quad \quad \mathcal{I}(h(i) == h(k)) \mathcal{I}(h(j) == h(d+k))  \mathcal{I}(h(i') == h(k')) \mathcal{I}(h(j') == h(d+k')) ) )\\
    \end{split}
\end{equation}

\begin{equation}
\begin{split}
    &\mathbb{V}(\widehat{\ip{x}{y}}) = \mathbb{E} \\ &  ((\sum_{k=1}^d \quad \sum_{i=1, \mathcal{C}(i) \neq \mathcal{C}(k) }^n  \quad \sum_{j=1, \mathcal{C}(j) \neq \mathcal{C}(d+k)}^n  \quad  \sum_{k'=1}^d \quad \sum_{i'=1, \mathcal{C}(i') \neq \mathcal{C}(k') }^n  \quad  \sum_{j'=1, \mathcal{C}(j') \neq \mathcal{C}(d + k')}^n \\
    & \quad \quad \theta_i \theta_j  \theta_{i'} \theta_{j'} \\
    & \quad \quad g(k) g(i) g(d+k) g(j) g(k') g(i') g(d+k') g(j')\\
    & \quad \quad \mathcal{I}(h(i) == h(k)) \mathcal{I}(h(j) == h(d+k))  \mathcal{I}(h(i') == h(k')) \mathcal{I}(h(j') == h(d+k')) ) )\\
    \end{split}
\end{equation}
